# Supplementary material for: Not Just Pretty Pictures: Toward Interventional Data Augmentation Using Text-to-Image Generators
Source: arXiv:2212.11237 source file (2024-06-03)
Supplement: Supplementary file 2 [file alternative_training.tex]

\begin{table}
\centering
\caption{PACS SDG result with contrastive training}
\label{tab:contrastive_pacs_app}
\resizebox{0.65\linewidth}{!}{\begin{tabular}{l|cccc|c} 
\toprule
 & Art & Photo & Sketch & Cartoon & Average  \\ 
\hline
ERM & $65.27$ & $39.0$ & $49.1$ & $71.65$ & $56.26$  \\
SDEdit(H/CE) & $78.49$ & $71.46$ & $\textbf{75.28}$ & $77.09$ & $\textbf{75.58}$ \\
SDEdit(H/COS) & $\textbf{81.35}$ & $\textbf{72.16}$ & $70.37$ & $77.36$ & $75.31$ \\
SDEdit(H/L2) & $81.24$ & $67.82$ & $71.49$ & $\textbf{77.92}$ & $74.62$  \\
\bottomrule
\end{tabular}}
\end{table}
