# Supplementary material for: Not Just Pretty Pictures: Toward Interventional Data Augmentation Using Text-to-Image Generators
Source: arXiv:2212.11237 source file (2024-06-03)
Supplement: Supplementary file 3 [file generation_expense.tex]

\begin{table}
\centering
\caption{Computational Expense of Image Manipulation}
\label{tab:generation_expense}
\resizebox{1.0\linewidth}{!}{\begin{tabular}{lcc} 
\toprule
                 & Minimum Memory Usage(GB) & Computational Time(sec/sample)  \\
\hline
% VQGAN-CLIP       & 6.5              & 5                          \\
Stable Diffusion & 6.5               & 1.5                          \\
\bottomrule
\end{tabular}}
\end{table}
